# Supplementary material for: End-to-End Information Extraction by Character-Level Embedding and Multi-Stage Attentional U-Net
Source: arXiv:2106.00952 source file (2021-09-09)
Supplement: Supplementary file 1 [file supplemental.tex]

\begin{figure}[h]
\centering
\includegraphics[width=0.9\textwidth]{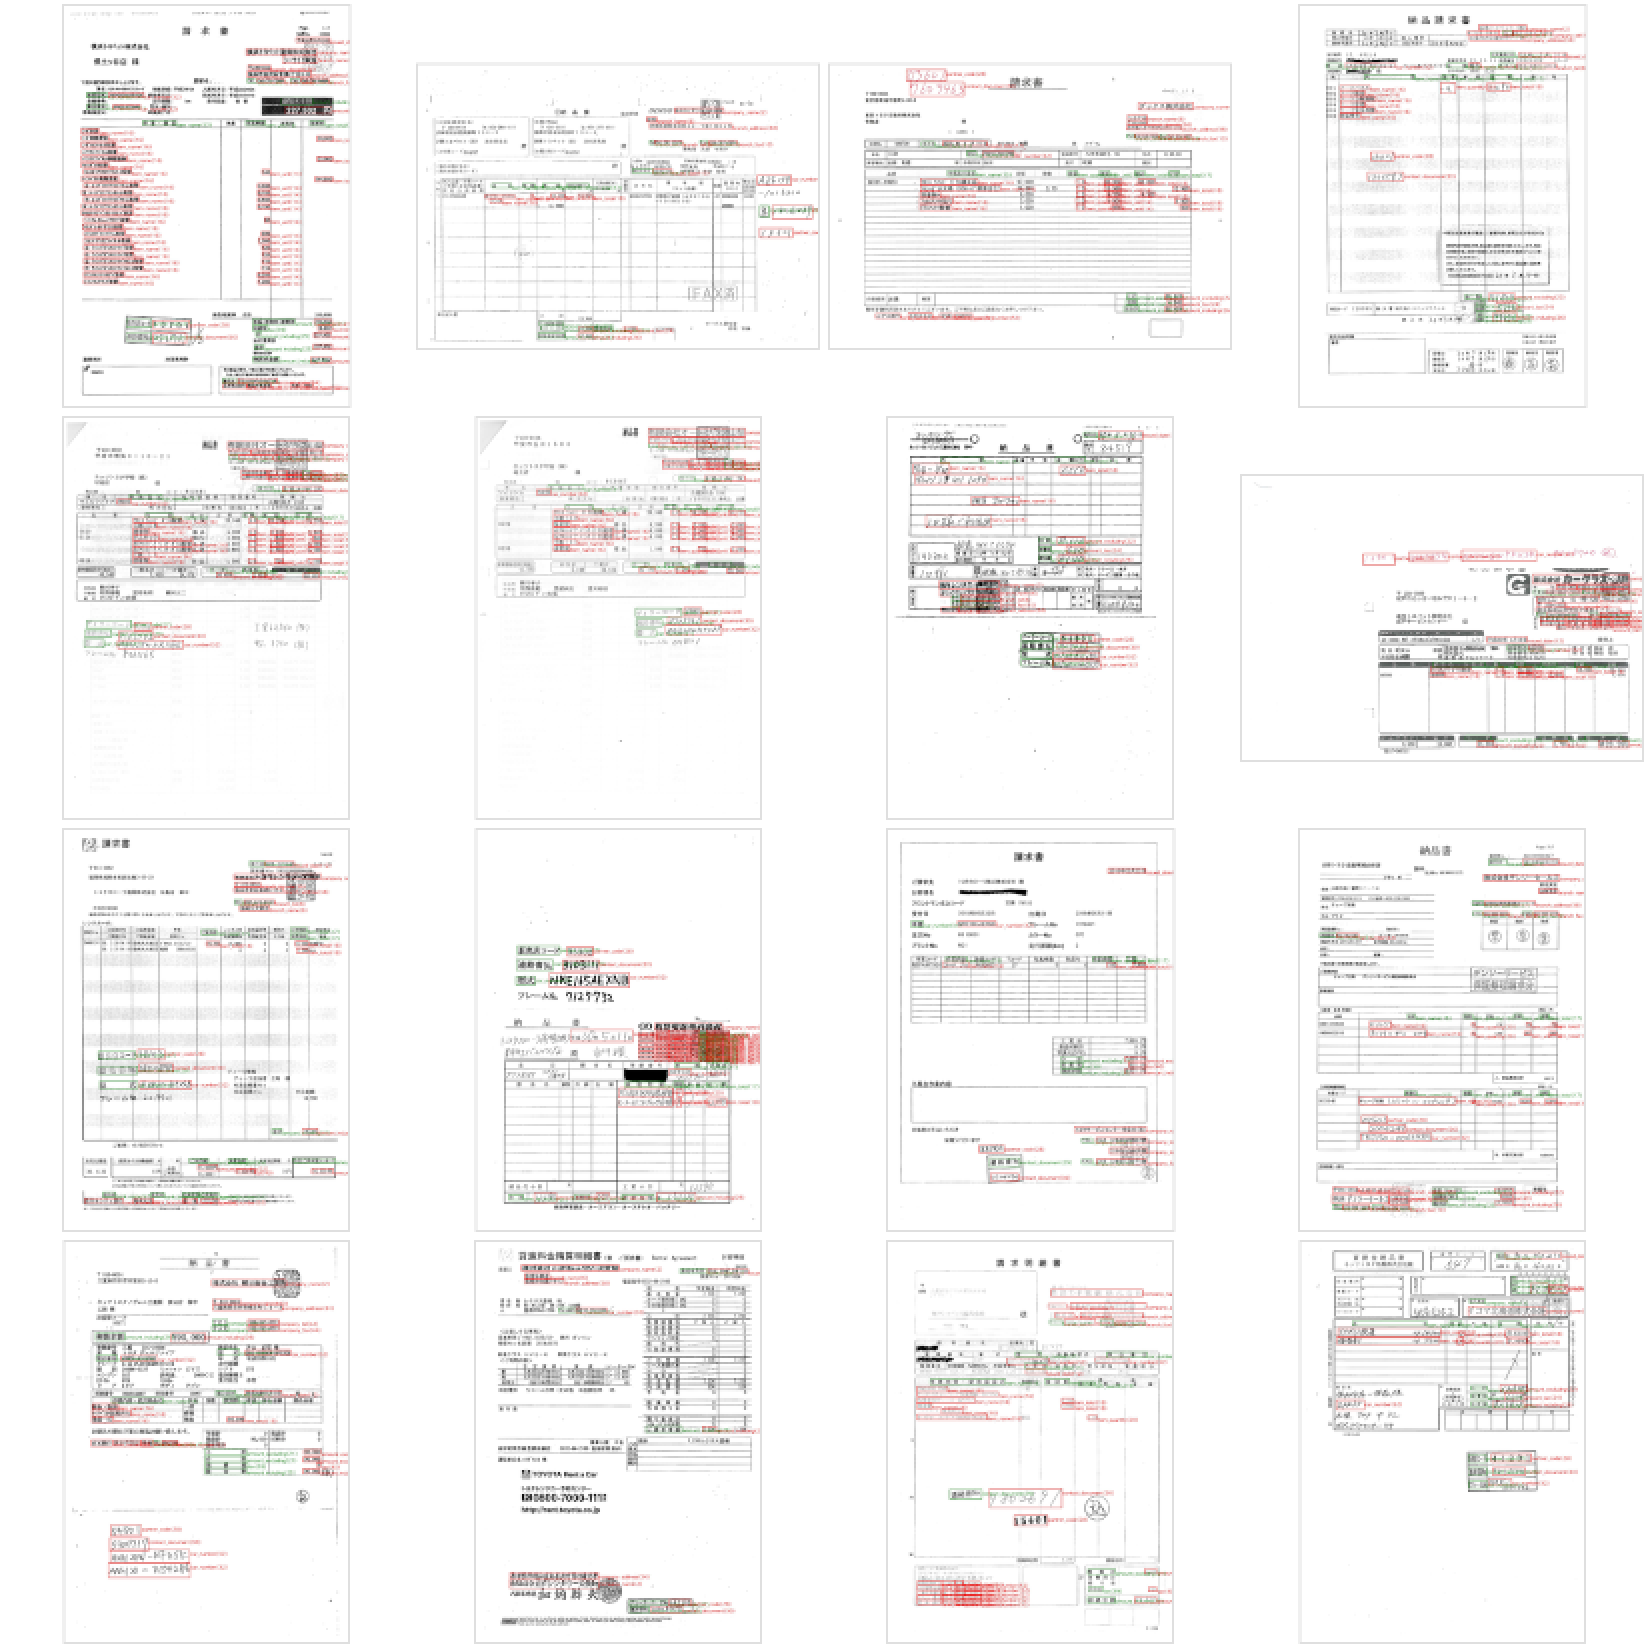}
\caption{Sample documents in the Japanese invoice dataset. \small{\textit{Green box denotes the key field, red box denotes the value field}}}
\label{fig:toyota_dataset}
\end{figure}

\begin{figure}[h]
\centering
\includegraphics[width=0.9\textwidth]{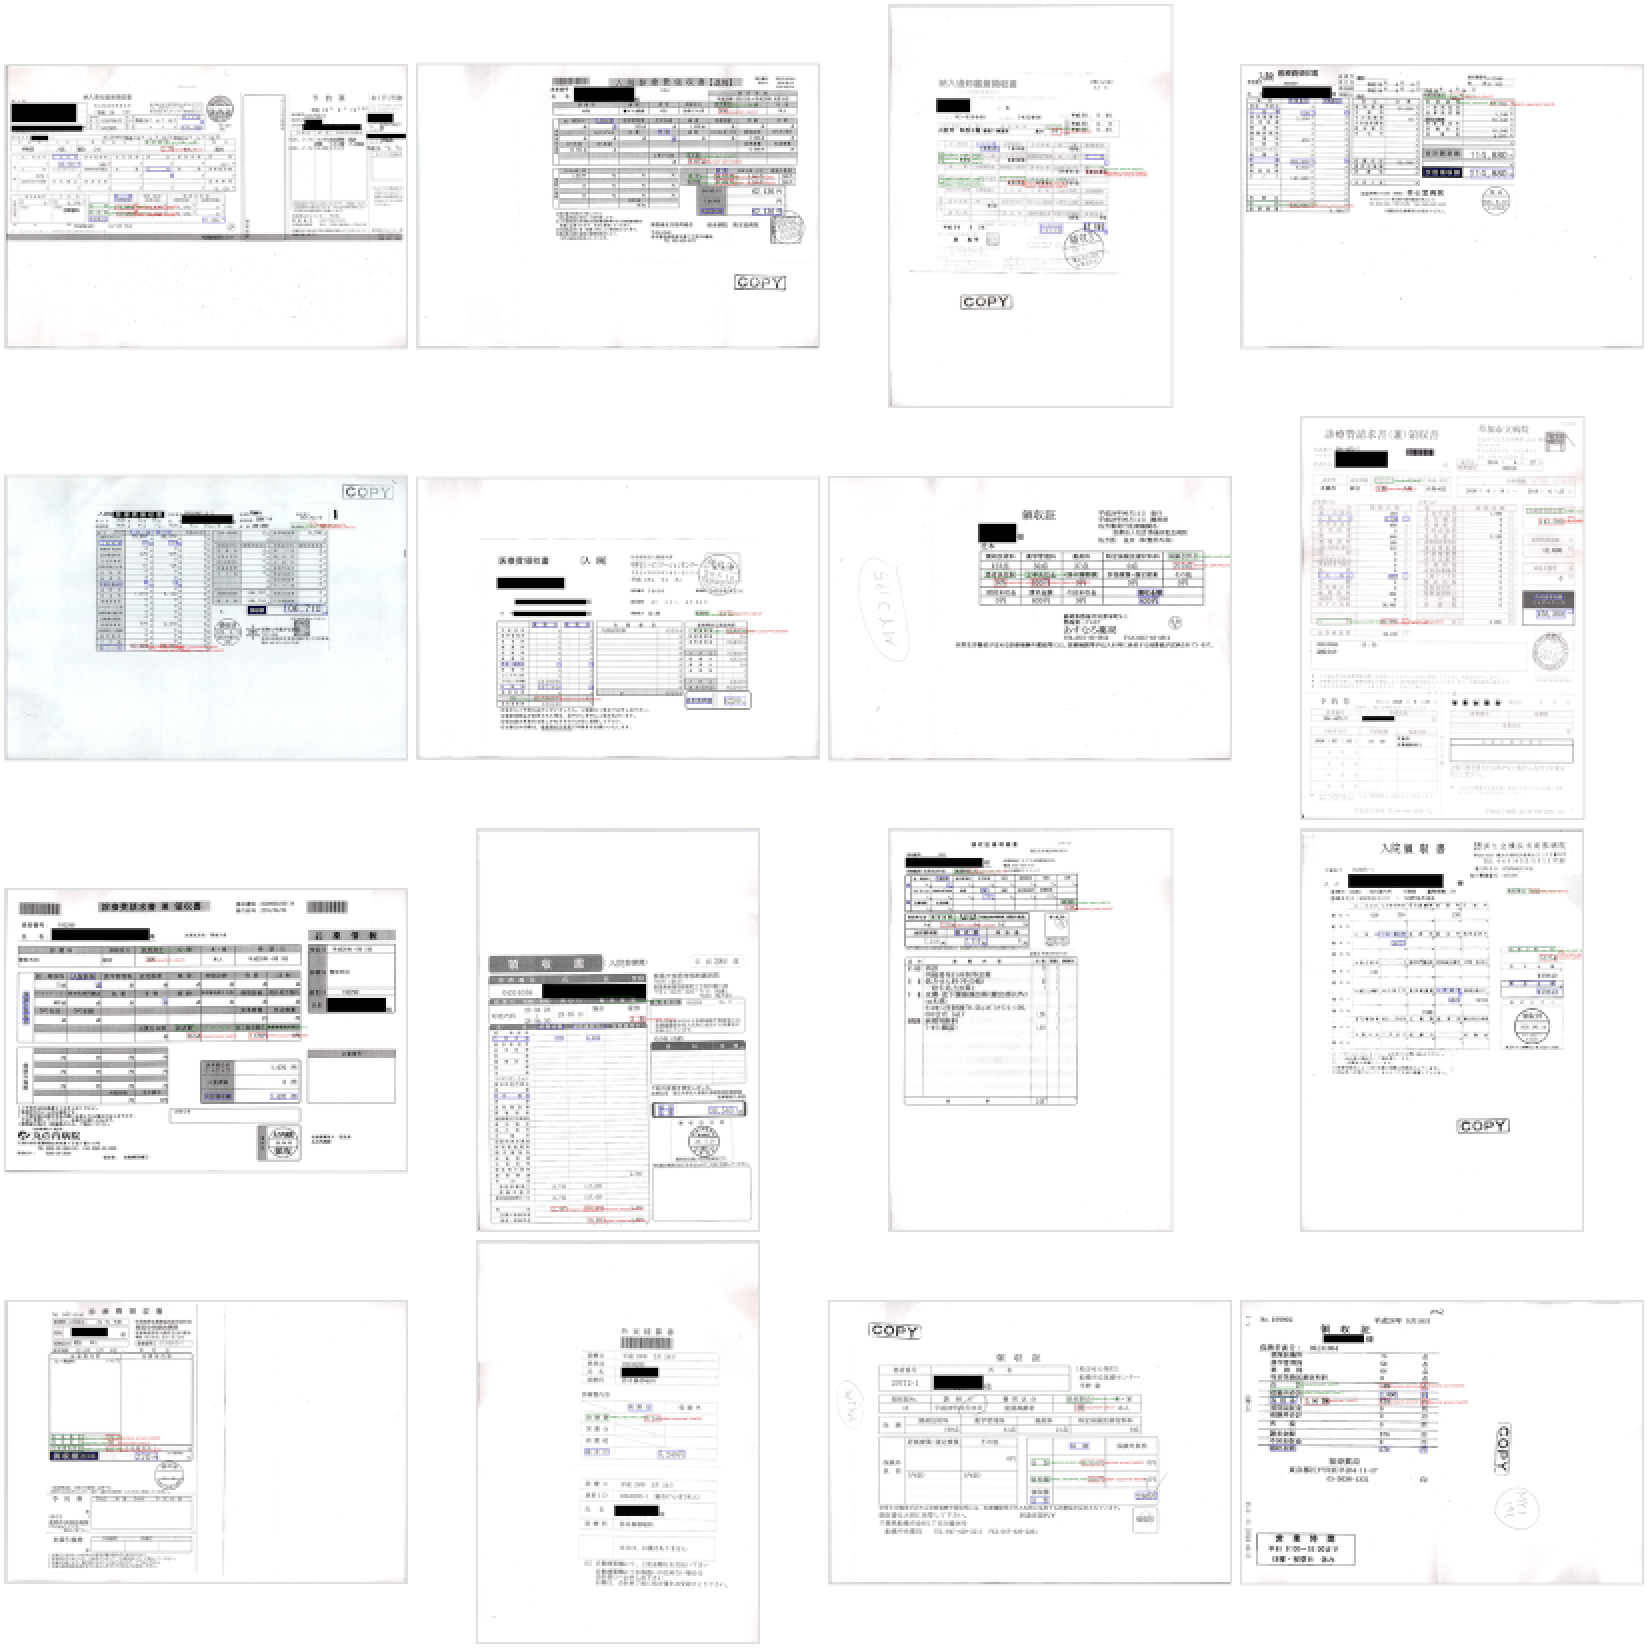}
\caption{Sample documents in the Japanese medical receipt dataset}
\label{fig:daiichi_dataset}
\end{figure}

\begin{figure}[h]
\centering
\includegraphics[width=0.9\textwidth]{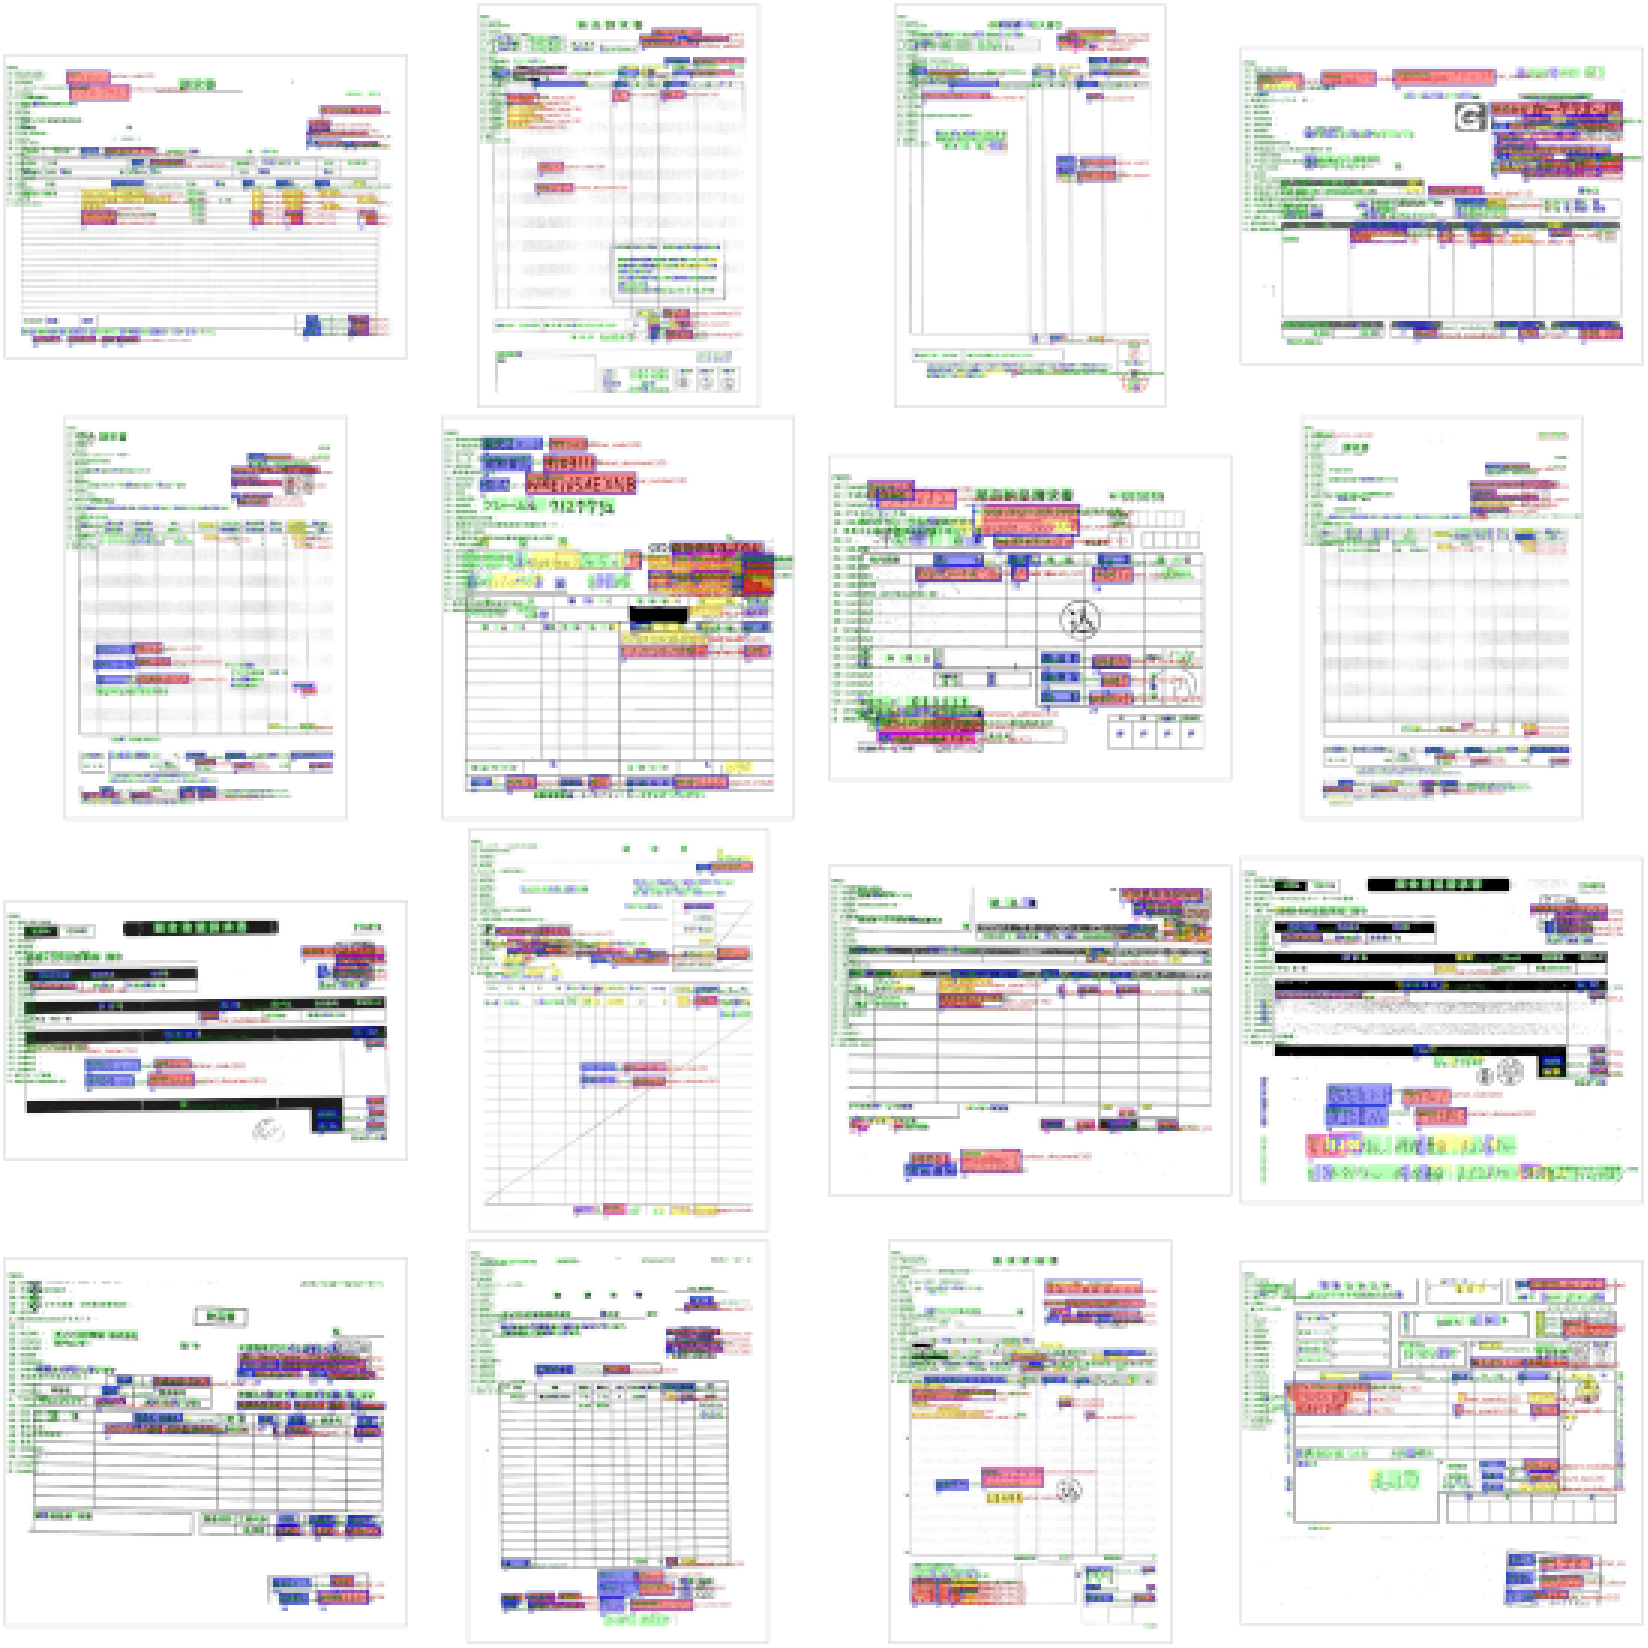}
\caption{Sample outputs on the Japanese invoice dataset. \small{\textit{Segmented key mask is presented in blue, value mask is presented in red}}}
\label{fig:toyota_output}
\end{figure}
